# Supplementary material for: Energy spectra of non-local internal gravity wave turbulence
Source: arXiv:2309.06181 ancillary file (2023-11-27)
Supplement: Supplementary file 1 [file SM_Lanchon_2024.pdf]

# —Supplemental Material—
# Energy spectra of non-local internal gravity wave turbulence

Nicolas Lanchon[1] and Pierre-Philippe Cortet[1,*]

[1] *Université Paris-Saclay, CNRS, FAST, 91405 Orsay, France*

In this Supplemental Material, we provide the details of several analytical calculations whose results are used in the Letter.

## I. CONSERVATION OF THE RATIO $\omega^*_{\mathbf{k}}/|k_z|$ BY "INDUCED DIFFUSION" RESONANT TRIADS

We consider a resonant triad of internal gravity waves of wavectors $\mathbf{k}$, $\mathbf{p}$ and $\mathbf{q}$ and respective non-dimensional frequencies $\omega^*_{\mathbf{k}}$, $\omega^*_{\mathbf{p}}$ and $\omega^*_{\mathbf{q}}$ which verify the resonance conditions

$$\mathbf{k} = \mathbf{p} + \mathbf{q}\,, \tag{1}$$

$$\omega^*_{\mathbf{k}} = \omega^*_{\mathbf{p}} + \omega^*_{\mathbf{q}}\,. \tag{2}$$

As in the Letter, we consider waves in the strong anisotropy limit, i.e. with $k_\perp \ll |k_z|$ and $\omega^*_{\mathbf{k}} \simeq k_\perp/|k_z|$ (same for $\mathbf{p}$ and $\mathbf{q}$).

In this section, we show that, if the resonant triad additionally verifies the "induced diffusion" conditions

$$\omega^*_{\mathbf{q}} \ll \omega^*_{\mathbf{p}} \sim \omega^*_{\mathbf{k}}\,, \tag{3}$$

$$|\mathbf{q}| \ll |\mathbf{p}| \sim |\mathbf{k}|\,, \tag{4}$$

the ratio of the wave frequency to the vertical component of the wavevector is conserved, i.e. that

$$\frac{\omega^*_{\mathbf{k}}}{|k_z|} = \frac{\omega^*_{\mathbf{p}}}{|p_z|} = \frac{\omega^*_{\mathbf{q}}}{|q_z|}\,. \tag{5}$$

To demonstrate this result, we first use the fact that the wavenumber $|\mathbf{q}|$ is very small [according to Eq. (4)] to write the expansion

$$\omega^*_{\mathbf{p}+\mathbf{q}} - \omega^*_{\mathbf{p}} = \mathbf{q}\cdot\nabla\omega^*_{\mathbf{p}} \tag{6}$$

from which it follows that

$$\omega^*_{\mathbf{q}} = \mathbf{q}_\perp\cdot\nabla_\perp\omega^*_{\mathbf{p}} + q_z\frac{\partial\omega^*_{\mathbf{p}}}{\partial p_z}\,, \tag{7}$$

where $\mathbf{q}_\perp$ and $\nabla_\perp$ are the projections of the wave vector $\mathbf{q}$ (same for $\mathbf{k}$ and $\mathbf{p}$) and of the vector differential operator on the plane normal to gravity, respectively. Considering the strong anisotropy hypothesis, we can estimate the order of magnitude of the two terms of the right hand side (rhs) of Eq. (7) as

$$|\mathbf{q}_\perp\cdot\nabla_\perp\omega^*_{\mathbf{p}}| \;\sim \tfrac{q_\perp}{|p_z|}\,, \tag{8}$$

$$\left|q_z\frac{\partial\omega^*_{\mathbf{p}}}{\partial p_z}\right| \sim \tfrac{|q_z|p_\perp}{|p_z|^2}\,, \tag{9}$$

such that

$$\frac{|\mathbf{q}_\perp\cdot\nabla_\perp\omega^*_{\mathbf{p}}|}{|q_z\partial\omega^*_{\mathbf{p}}/\partial p_z|} \sim \frac{|p_z|}{p_\perp}\frac{q_\perp}{|q_z|} \sim \frac{\omega^*_{\mathbf{q}}}{\omega^*_{\mathbf{p}}} \ll 1\,, \tag{10}$$

the last inequality following from Eq. (3).

* pierre-philippe.cortet@universite-paris-saclay.fr

Using (10) and the strong anisotropy condition in Eq. (7), we can further demonstrate that

$$\frac{p_\perp}{p_z^2} = -\,\mathrm{sgn}(p_z q_z)\frac{q_\perp}{q_z^2}\,. \tag{11}$$

Since $p_\perp/p_z^2$ and $q_\perp/q_z^2$ are both positive, Eq. (11) implies that $p_z q_z < 0$. Finally, we obtain that, under the "induced diffusion" hypotheses,

$$\frac{p_\perp}{p_z^2} = \frac{k_\perp}{k_z^2} = \frac{q_\perp}{q_z^2}\,, \tag{12}$$

which is equivalent to Eq. (5).

## II. EXPRESSION OF $T_{\mathbf{kpq}}$ IN THE INDUCED DIFFUSION LIMIT

In this section, we derive a simplified expression for the transfer coefficient $T_{\mathbf{kpq}}$ for a resonant triad [i.e., verifying Eqs. (1) and (2)] in the induced diffusion limit defined by Eqs. (3) and (4).

First, we recall the general expression of $T_{\mathbf{kpq}}$

$$T_{\mathbf{kpq}} = \left(\tilde{k}_\perp + \tilde{p}_\perp + \tilde{q}_\perp\right)^2 \frac{\left(k_z^2 - p_z q_z\right)^2}{16|k_z p_z q_z| k_\perp p_\perp q_\perp} \left(\frac{k_\perp^2 - \tilde{p}_\perp \tilde{q}_\perp}{k_z^2 - p_z q_z} k_z - \frac{p_\perp^2}{p_z} - \frac{q_\perp^2}{q_z}\right)^2\,, \tag{13}$$

where $\tilde{m}_\perp = \mathrm{sgn}(m_z) m_\perp$ (with $\mathbf{m} = \mathbf{k}$, $\mathbf{p}$ or $\mathbf{q}$). The rhs of Eq. (13) is the product of three terms. In the induced diffusion limit, the first two terms can easily be simplified, leading to the expression

$$T_{\mathbf{kpq}} \simeq \frac{1}{4}\frac{k_z^2}{|q_z| q_\perp} \left(\frac{k_\perp^2 - \tilde{p}_\perp \tilde{q}_\perp}{k_z^2 - p_z q_z} k_z - \frac{p_\perp^2}{p_z} - \frac{q_\perp^2}{q_z}\right)^2\,. \tag{14}$$

Then, to simplify the last term, we first use Eqs. (3) and (4) to remark that $q_\perp^2/q_z$ is very small compared to $p_\perp^2/p_z$, leading to

$$T_{\mathbf{kpq}} \simeq \frac{1}{4}\frac{k_z^2}{|q_z| q_\perp} \left(\frac{k_\perp^2 - \tilde{p}_\perp \tilde{q}_\perp}{k_z^2 - p_z q_z} k_z - \frac{p_\perp^2}{p_z}\right)^2\,. \tag{15}$$

Once again using Eqs. (3) and (4), we can also show that $k_\perp^2 \gg |\tilde{p}_\perp \tilde{q}_\perp|$ and $k_z^2 \gg |p_z q_z|$. We thus obtain that

$$T_{\mathbf{kpq}} \simeq \frac{1}{4}\frac{k_z^2}{|q_z| q_\perp} \left(\frac{k_\perp^2}{k_z} - \frac{p_\perp^2}{p_z}\right)^2 \tag{16}$$

which can be simplified in

$$T_{\mathbf{kpq}} \simeq \frac{1}{4|q_z| q_\perp} \left(k_\perp^2 - p_\perp^2\right)^2\,, \tag{17}$$

since $p_z = k_z - q_z \simeq k_z$.

Finally, we introduce the angle $\varphi_{\mathbf{kq}}$ between the projections $\mathbf{k}_\perp$ and $\mathbf{q}_\perp$ on the horizontal plane, normal to gravity, of the wavevectors $\mathbf{k}$ and $\mathbf{q}$, respectively. This angle verifies the relation

$$\cos(\varphi_{\mathbf{kq}}) = \frac{k_\perp^2 + q_\perp^2 - p_\perp^2}{2 k_\perp q_\perp} \simeq \frac{k_\perp^2 - p_\perp^2}{2 k_\perp q_\perp}\,, \tag{18}$$

which leads to a simple expression of $T_{\mathbf{kpq}}$ in the induced diffusion limit

$$T_{\mathbf{kpq}} \simeq \frac{q_\perp}{|q_z|} k_\perp^2 \cos^2(\varphi_{\mathbf{kq}})\,. \tag{19}$$

In the same way, it can be shown, still in the induced diffusion limit defined by Eqs. (3) and (4) and on the relevant resonant manifold defined by $\mathbf{p} = \mathbf{k} + \mathbf{q}$ and $\omega_{\mathbf{p}}^* = \omega_{\mathbf{k}}^* + \omega_{\mathbf{q}}^*$, that

$$T_{\mathbf{pkq}} \simeq \frac{q_\perp}{|q_z|} k_\perp^2 \cos^2(\varphi_{\mathbf{kq}})\,. \tag{20}$$

## III. SIMPLIFICATION OF THE KINETIC EQUATION FOLLOWING ITS RESTRICTION TO INDUCED DIFFUSION TRIADS

In this section, we derive a simplified expression of the kinetic equation assuming that the collision integral is dominated by the resonant triads in the induced diffusion limit, defined by $\omega^*_{\mathbf{q}} \ll \omega^*_{\mathbf{k}} \sim \omega^*_{\mathbf{p}}$ and $|\mathbf{q}| \ll |\mathbf{k}| \sim |\mathbf{p}|$.

First, we recall the general expression of the kinetic equation

$$\begin{aligned} \frac{\partial n_{\mathbf{k}}}{\partial t} \propto & \int T_{\mathbf{kpq}}(n_{\mathbf{p}}n_{\mathbf{q}} - n_{\mathbf{k}}n_{\mathbf{p}} - n_{\mathbf{k}}n_{\mathbf{q}})\delta^{\mathbf{k}}_{\mathbf{pq}}\delta(\Omega^{\mathbf{k}}_{\mathbf{pq}})d\mathbf{p}d\mathbf{q} \\ & - \int T_{\mathbf{pkq}}(n_{\mathbf{k}}n_{\mathbf{q}} - n_{\mathbf{p}}n_{\mathbf{k}} - n_{\mathbf{p}}n_{\mathbf{q}})\delta^{\mathbf{p}}_{\mathbf{kq}}\delta(\Omega^{\mathbf{p}}_{\mathbf{kq}})d\mathbf{p}d\mathbf{q} \\ & - \int T_{\mathbf{qpk}}(n_{\mathbf{p}}n_{\mathbf{k}} - n_{\mathbf{q}}n_{\mathbf{p}} - n_{\mathbf{q}}n_{\mathbf{k}})\delta^{\mathbf{q}}_{\mathbf{pk}}\delta(\Omega^{\mathbf{q}}_{\mathbf{pk}})d\mathbf{p}d\mathbf{q}\,, \end{aligned} \tag{21}$$

where $\delta^{\mathbf{k}}_{\mathbf{pq}} = \delta(\mathbf{k}-\mathbf{p}-\mathbf{q})$, $\Omega^{\mathbf{k}}_{\mathbf{pq}} = \omega^*_{\mathbf{k}} - \omega^*_{\mathbf{p}} - \omega^*_{\mathbf{q}}$ and $T_{\mathbf{kpq}}$ is defined by Eq. (13).

We start by neglecting the third term of the rhs of Eq. (21) since the resonant manifold corresponding to $T_{\mathbf{qpk}}$ does not involve induced diffusion triads (i.e. triads verifying Eqs. (3) and (4)). Then, assuming the induced diffusion triads completely dominate the energy exchanges allows us to restrict to small wavenumbers the integral over $\mathbf{q}$ in Eq. (21). In practice, we introduce a cutoff wavenumber $\tilde{q}$, verifying $\tilde{q} \ll |\mathbf{k}|$ such that, from now on, the integration over $\mathbf{q}$ is restricted to the domain $|\mathbf{q}| \leq \tilde{q}$.

Next, assuming that the wave action spectrum is steep enough and considering the scale separation present in the induced diffusion triads, we can write that $n_{\mathbf{q}} \gg n_{\mathbf{p}} \sim n_{\mathbf{k}}$. The terms $n_{\mathbf{k}}n_{\mathbf{p}}$ can therefore be neglected in the kinetic equation (21) leading to the simplified equation

$$\frac{\partial n_{\mathbf{k}}}{\partial t} \propto \int (Q_{\mathbf{kpq}} - Q_{\mathbf{pkq}})\, d\mathbf{p}d\mathbf{q}\,, \tag{22}$$

with

$$Q_{\mathbf{kpq}} = T_{\mathbf{kpq}}n_{\mathbf{q}}(n_{\mathbf{p}} - n_{\mathbf{k}})\delta^{\mathbf{k}}_{\mathbf{pq}}\delta(\Omega^{\mathbf{k}}_{\mathbf{pq}})\,. \tag{23}$$

Then, following a method used by Galtier in Ref. [1] for simplifying the kinetic equation of inertial wave turbulence, we multiply Eq. (22) by an arbitrary function $f$ of $\mathbf{k}$ (which is zero outside a finite domain of interest) and integrate the result with respect to $\mathbf{k}$, which leads to

$$\int f(\mathbf{k})\frac{\partial n_{\mathbf{k}}}{\partial t}d\mathbf{k} \propto \int f(\mathbf{k})(Q_{\mathbf{kpq}} - Q_{\mathbf{pkq}})d\mathbf{k}d\mathbf{p}d\mathbf{q}\,. \tag{24}$$

This last equation can be transformed into

$$\int f(\mathbf{k})\frac{\partial n_{\mathbf{k}}}{\partial t}d\mathbf{k} \propto -\int f(\mathbf{p})(Q_{\mathbf{kpq}} - Q_{\mathbf{pkq}})d\mathbf{k}d\mathbf{p}d\mathbf{q}\,, \tag{25}$$

$$\propto \frac{1}{2}\int (f(\mathbf{k}) - f(\mathbf{p}))(Q_{\mathbf{kpq}} - Q_{\mathbf{pkq}})d\mathbf{k}d\mathbf{p}d\mathbf{q}\,. \tag{26}$$

Eq. (25) is obtained from Eq. (24) by exchanging the roles of $\mathbf{k}$ and $\mathbf{p}$. We further remark the fact that

$$f(\mathbf{k}) - f(\mathbf{p}) \simeq q_i\frac{\partial f}{\partial k_i}\,, \quad \text{when} \quad \mathbf{k} = \mathbf{p} + \mathbf{q}\,, \tag{27}$$

and

$$f(\mathbf{k}) - f(\mathbf{p}) \simeq -q_i\frac{\partial f}{\partial k_i}\,, \quad \text{when} \quad \mathbf{p} = \mathbf{k} + \mathbf{q}\,, \tag{28}$$

where we use the Einstein summation convention with $i = x$, $y$, and $z$. These last two equations combined to integrations by parts leads to

$$\int f(\mathbf{k})\frac{\partial n_{\mathbf{k}}}{\partial t}d\mathbf{k} \propto -\frac{1}{2}\int f(\mathbf{k})q_i\frac{\partial}{\partial k_i}(Q_{\mathbf{kpq}} + Q_{\mathbf{pkq}})d\mathbf{k}d\mathbf{p}d\mathbf{q}\,. \tag{29}$$

Finally, since Eq. (29) has to be verified for any regular function $f$ of $\mathbf{k}$, we must have

$$\frac{\partial n_{\mathbf{k}}}{\partial t} \propto -\int q_i \frac{\partial}{\partial k_i}(Q_{\mathbf{kpq}} + Q_{\mathbf{pkq}}) d\mathbf{p} d\mathbf{q} \,. \tag{30}$$

Besides, since $|\mathbf{q}| = |\mathbf{k} - \mathbf{p}|$ is very small in the induced diffusion limit, using Eqs. (19) and (20) we can simplify Eq. (23) into

$$Q_{\mathbf{kpq}} \simeq -T_{\mathbf{kpq}} n_{\mathbf{q}} q_j \frac{\partial n_{\mathbf{k}}}{\partial k_j} \delta^{\mathbf{k}}_{\mathbf{pq}} \delta(\Omega^{\mathbf{k}}_{\mathbf{pq}}) \,, \tag{31}$$

$$Q_{\mathbf{pkq}} \simeq -T_{\mathbf{kpq}} n_{\mathbf{q}} q_j \frac{\partial n_{\mathbf{k}}}{\partial k_j} \delta^{\mathbf{p}}_{\mathbf{kq}} \delta(\Omega^{\mathbf{p}}_{\mathbf{kq}}) \,, \tag{32}$$

such that Eq. (30) becomes

$$\frac{\partial n_{\mathbf{k}}}{\partial t} \propto \frac{\partial}{\partial k_i} D_{ij}(\mathbf{k}) \frac{\partial n_{\mathbf{k}}}{\partial k_j} \,, \tag{33}$$

with

$$D_{ij}(\mathbf{k}) = \int q_i q_j n_{\mathbf{q}} T_{\mathbf{kpq}} \left( \delta^{\mathbf{k}}_{\mathbf{pq}} \delta(\Omega^{\mathbf{k}}_{\mathbf{pq}}) + \delta^{\mathbf{p}}_{\mathbf{kq}} \delta(\Omega^{\mathbf{p}}_{\mathbf{kq}}) \right) d\mathbf{p} d\mathbf{q} \,. \tag{34}$$

We use here the Einstein summation convention for the indices $i$ and $j$ running over the values $x$, $y$, and $z$. Finally, integrating over $\mathbf{p}$, considering again the fact the components of $\mathbf{q}$ are very small compared to those of $\mathbf{k}$ and applying the expansion of Eq. (6) in $\delta(\Omega^{\mathbf{p}}_{\mathbf{kq}})$, we obtain that

$$D_{ij}(\mathbf{k}) = 2 \int q_i q_j n_{\mathbf{q}} T \, \delta\left( q_z \frac{k_\perp}{k_z^2} - \frac{q_\perp}{q_z} \right) d\mathbf{q} \,, \tag{35}$$

with

$$T = T_{\mathbf{kpq}} \simeq \frac{q_\perp}{|q_z|} k_\perp^2 \cos^2(\varphi_{\mathbf{kq}}) \,. \tag{36}$$

One can note that the "induced diffusion" relation $k_\perp / k_z^2 \simeq q_\perp / q_z^2$ naturally emerges here in the delta function of Eq. (35).

## IV. THE SIMPLIFIED KINETIC EQUATION IN CYLINDRICAL COORDINATES

In the following, we search to rewrite Eq. (33) using cylindrical coordinates. Let us first write its developed expression

$$\frac{\partial n_{\mathbf{k}}}{\partial t} \propto \int q_i \frac{\partial}{\partial k_i} \frac{q_\perp}{|q_z|} k_\perp^2 \cos^2(\varphi_{\mathbf{k}} - \varphi_{\mathbf{q}}) n_{\mathbf{q}} \delta\left( q_z \frac{k_\perp}{k_z^2} - \frac{q_\perp}{q_z} \right) q_j \frac{\partial n_{\mathbf{k}}}{\partial k_j} q_\perp dq_\perp d\varphi_{\mathbf{q}} dq_z, \tag{37}$$

where $\varphi_{\mathbf{q}}$ and $\varphi_{\mathbf{k}}$ are the angles, with respect to an arbitrary reference, of the projections in the horizontal plane of $\mathbf{q}$ and $\mathbf{k}$, respectively ($\varphi_{\mathbf{kq}} = \varphi_{\mathbf{k}} - \varphi_{\mathbf{q}}$).

Let us first remark that

$$\frac{\partial}{\partial k_x} = \cos\varphi_{\mathbf{k}} \frac{\partial}{\partial k_\perp} - \frac{\sin\varphi_{\mathbf{k}}}{k_\perp} \frac{\partial}{\partial \varphi_{\mathbf{k}}} \,, \tag{38}$$

$$\frac{\partial}{\partial k_y} = \sin\varphi_{\mathbf{k}} \frac{\partial}{\partial k_\perp} + \frac{\cos\varphi_{\mathbf{k}}}{k_\perp} \frac{\partial}{\partial \varphi_{\mathbf{k}}} \,, \tag{39}$$

such that for an arbitrary function $f$

$$q_i \frac{\partial f}{\partial k_i} = q_\perp \cos(\varphi_{\mathbf{k}} - \varphi_{\mathbf{q}}) \frac{\partial f}{\partial k_\perp} - \frac{q_\perp}{k_\perp} \sin(\varphi_{\mathbf{k}} - \varphi_{\mathbf{q}}) \frac{\partial f}{\partial \varphi_{\mathbf{k}}} + q_z \frac{\partial f}{\partial k_z} \,. \tag{40}$$

Applying this relation to the wave action spectrum $n_{\mathbf{k}}$, which is independent of $\varphi_{\mathbf{k}}$ due to statistical axisymmetry, it comes

$$q_j \frac{\partial n_{\mathbf{k}}}{\partial k_j} = q_\perp \cos(\varphi_{\mathbf{k}} - \varphi_{\mathbf{q}}) \frac{\partial n_{\mathbf{k}}}{\partial k_\perp} + q_z \frac{\partial n_{\mathbf{k}}}{\partial k_z} \,, \tag{41}$$

and we can write

$$\begin{aligned}
\frac{\partial n_{\mathbf{k}}}{\partial t} \propto & \frac{\partial}{\partial k_\perp} \int \frac{q_\perp^2}{|q_z|} k_\perp^2 \cos^3(\varphi_{\mathbf{k}} - \varphi_{\mathbf{q}}) n_{\mathbf{q}} \delta\!\left(q_z \frac{k_\perp}{k_z^2} - \frac{q_\perp}{q_z}\right) \left(q_\perp \cos(\varphi_{\mathbf{k}} - \varphi_{\mathbf{q}}) \frac{\partial n_{\mathbf{k}}}{\partial k_\perp} + q_z \frac{\partial n_{\mathbf{k}}}{\partial k_z}\right) q_\perp dq_\perp d\varphi_{\mathbf{q}} dq_z \\
& - \int \sin(\varphi_{\mathbf{k}} - \varphi_{\mathbf{q}}) \frac{\partial}{\partial \varphi_{\mathbf{k}}} \frac{q_\perp^2}{|q_z|} k_\perp \cos^2(\varphi_{\mathbf{k}} - \varphi_{\mathbf{q}}) n_{\mathbf{q}} \delta\!\left(q_z \frac{k_\perp}{k_z^2} - \frac{q_\perp}{q_z}\right) \left(q_\perp \cos(\varphi_{\mathbf{k}} - \varphi_{\mathbf{q}}) \frac{\partial n_{\mathbf{k}}}{\partial k_\perp} + q_z \frac{\partial n_{\mathbf{k}}}{\partial k_z}\right) q_\perp dq_\perp d\varphi_{\mathbf{q}} dq_z \\
& + \frac{\partial}{\partial k_z} \int \frac{q_\perp q_z}{|q_z|} k_\perp^2 \cos^2(\varphi_{\mathbf{k}} - \varphi_{\mathbf{q}}) n_{\mathbf{q}} \delta\!\left(q_z \frac{k_\perp}{k_z^2} - \frac{q_\perp}{q_z}\right) \left(q_\perp \cos(\varphi_{\mathbf{k}} - \varphi_{\mathbf{q}}) \frac{\partial n_{\mathbf{k}}}{\partial k_\perp} + q_z \frac{\partial n_{\mathbf{k}}}{\partial k_z}\right) q_\perp dq_\perp d\varphi_{\mathbf{q}} dq_z \,.
\end{aligned} \tag{42}$$

This last equation can be developed in

$$\begin{aligned}
\frac{\partial n_{\mathbf{k}}}{\partial t} \propto & \frac{\partial}{\partial k_\perp} \int \frac{q_\perp^4}{|q_z|} k_\perp^2 \cos^4(\varphi_{\mathbf{k}} - \varphi_{\mathbf{q}}) n_{\mathbf{q}} \delta\!\left(q_z \frac{k_\perp}{k_z^2} - \frac{q_\perp}{q_z}\right) \frac{\partial n_{\mathbf{k}}}{\partial k_\perp} dq_\perp d\varphi_{\mathbf{q}} dq_z \\
& + \frac{\partial}{\partial k_\perp} \int \frac{q_\perp^3 q_z}{|q_z|} k_\perp^2 \cos^3(\varphi_{\mathbf{k}} - \varphi_{\mathbf{q}}) n_{\mathbf{q}} \delta\!\left(q_z \frac{k_\perp}{k_z^2} - \frac{q_\perp}{q_z}\right) \frac{\partial n_{\mathbf{k}}}{\partial k_z} dq_\perp d\varphi_{\mathbf{q}} dq_z \\
& + 3 \int \frac{q_\perp^4}{|q_z|} k_\perp \cos^2(\varphi_{\mathbf{k}} - \varphi_{\mathbf{q}}) \sin^2(\varphi_{\mathbf{k}} - \varphi_{\mathbf{q}}) n_{\mathbf{q}} \delta\!\left(q_z \frac{k_\perp}{k_z^2} - \frac{q_\perp}{q_z}\right) \frac{\partial n_{\mathbf{k}}}{\partial k_\perp} dq_\perp d\varphi_{\mathbf{q}} dq_z \\
& + 2 \int \frac{q_\perp^3 q_z}{|q_z|} k_\perp \cos(\varphi_{\mathbf{k}} - \varphi_{\mathbf{q}}) \sin^2(\varphi_{\mathbf{k}} - \varphi_{\mathbf{q}}) n_{\mathbf{q}} \delta\!\left(q_z \frac{k_\perp}{k_z^2} - \frac{q_\perp}{q_z}\right) \frac{\partial n_{\mathbf{k}}}{\partial k_z} dq_\perp d\varphi_{\mathbf{q}} dq_z \\
& + \frac{\partial}{\partial k_z} \int \frac{q_\perp^3 q_z}{|q_z|} k_\perp^2 \cos^3(\varphi_{\mathbf{k}} - \varphi_{\mathbf{q}}) n_{\mathbf{q}} \delta\!\left(q_z \frac{k_\perp}{k_z^2} - \frac{q_\perp}{q_z}\right) \frac{\partial n_{\mathbf{k}}}{\partial k_\perp} dq_\perp d\varphi_{\mathbf{q}} dq_z \\
& + \frac{\partial}{\partial k_z} \int \frac{q_\perp^2 q_z^2}{|q_z|} k_\perp^2 \cos^2(\varphi_{\mathbf{k}} - \varphi_{\mathbf{q}}) n_{\mathbf{q}} \delta\!\left(q_z \frac{k_\perp}{k_z^2} - \frac{q_\perp}{q_z}\right) \frac{\partial n_{\mathbf{k}}}{\partial k_z} dq_\perp d\varphi_{\mathbf{q}} dq_z \,.
\end{aligned} \tag{43}$$

Proceeding to the integration with respect to $\varphi_{\mathbf{q}}$, we obtain

$$\begin{aligned}
\frac{\partial n_{\mathbf{k}}}{\partial t} \propto & \frac{3\pi}{4} \frac{\partial}{\partial k_\perp} \int \frac{q_\perp^4}{|q_z|} k_\perp^2 n_{\mathbf{q}} \delta\!\left(q_z \frac{k_\perp}{k_z^2} - \frac{q_\perp}{q_z}\right) \frac{\partial n_{\mathbf{k}}}{\partial k_\perp} dq_\perp dq_z \\
& + 0 \\
& + \frac{3\pi}{4} \int \frac{q_\perp^4}{|q_z|} k_\perp n_{\mathbf{q}} \delta\!\left(q_z \frac{k_\perp}{k_z^2} - \frac{q_\perp}{q_z}\right) \frac{\partial n_{\mathbf{k}}}{\partial k_\perp} dq_\perp dq_z \\
& + 0 \\
& + 0 \\
& + \pi \frac{\partial}{\partial k_z} \int \frac{q_\perp^2 q_z^2}{|q_z|} k_\perp^2 n_{\mathbf{q}} \delta\!\left(q_z \frac{k_\perp}{k_z^2} - \frac{q_\perp}{q_z}\right) \frac{\partial n_{\mathbf{k}}}{\partial k_z} dq_\perp dq_z \,,
\end{aligned} \tag{44}$$

which can be simplified in

$$\frac{\partial n_{\mathbf{k}}}{\partial t} \propto \frac{3}{4} \frac{\partial}{\partial k_\perp} D_\perp \frac{\partial n_{\mathbf{k}}}{\partial k_\perp} + \frac{3}{4} \frac{D_\perp}{k_\perp} \frac{\partial n_{\mathbf{k}}}{\partial k_\perp} + \frac{\partial}{\partial k_z} D_z \frac{\partial n_{\mathbf{k}}}{\partial k_z} \,, \tag{45}$$

where

$$D_i = \int q_\perp^2 q_i^2 k_\perp^2 n_{\mathbf{q}} \delta\!\left(q_\perp - q_z^2 \frac{k_\perp}{k_z^2}\right) dq_\perp dq_z \,, \tag{46}$$

with $i = \perp$ or $i = z$.

Now using that

$$\frac{1}{k_\perp} \frac{\partial}{\partial k_\perp} k_\perp D_\perp \frac{\partial n_{\mathbf{k}}}{\partial k_\perp} = \frac{\partial}{\partial k_\perp} D_\perp \frac{\partial n_{\mathbf{k}}}{\partial k_\perp} + \frac{D_\perp}{k_\perp} \frac{\partial n_{\mathbf{k}}}{\partial k_\perp} \,, \tag{47}$$

Eq. (45) becomes

$$\frac{\partial n_{\mathbf{k}}}{\partial t} \propto \frac{3}{4}\frac{1}{k_\perp}\frac{\partial}{\partial k_\perp} k_\perp D_\perp \frac{\partial n_{\mathbf{k}}}{\partial k_\perp} + \frac{\partial}{\partial k_z} D_z \frac{\partial n_{\mathbf{k}}}{\partial k_z} \,. \tag{48}$$

## V. STEADY POWER LAW SOLUTION TO THE "INDUCED DIFFUSION" KINETIC EQUATION

In this section, we search for a steady power-law solution of the kinetic equation (48) of the form $n_{\mathbf{k}} \propto k_\perp^\alpha k_z^\beta$. For such a wave action spectrum, we have

$$D_z \frac{\partial n_{\mathbf{k}}}{\partial k_z} \sim \int q_\perp^{2+\alpha} q_z^{2+\beta} k_\perp^2 \delta\left( q_\perp - q_z^2 \frac{k_\perp}{k_z^2}\right) dq_\perp dq_z k_\perp^\alpha k_z^{\beta-1} \,, \tag{49}$$

$$\sim k_\perp^{4+2\alpha} k_z^{\beta-2\alpha-5} \int q_z^{6+2\alpha+\beta} dq_z \,, \tag{50}$$

such that the second term of the rhs of Eq. (48) cancels out for $\beta - 2\alpha = 5$.

Besides, we have

$$k_\perp D_\perp \frac{\partial n_{\mathbf{k}}}{\partial k_\perp} \sim \int q_\perp^{4+\alpha} q_z^{\beta} k_\perp^2 \delta\left( q_\perp - q_z^2 \frac{k_\perp}{k_z^2}\right) dq_\perp dq_z k_\perp^\alpha k_z^{\beta} \,, \tag{51}$$

$$\sim k_\perp^{6+2\alpha} k_z^{\beta-8-2\alpha} \int q_z^{8+2\alpha+\beta} dq_z \,, \tag{52}$$

such that the first term of the rhs of Eq. (48) cancels out for $\alpha = -3$, which implies $\beta = -1$ if one want to cancel out the second term at the same time.

In conclusion, we find that there is a single steady power-law solution to Eq. (48), which is given by

$$n_{\mathbf{k}} \sim k_\perp^{-3} k_z^{-1} \,. \tag{53}$$

[1] S. Galtier, *Physics of Wave Turbulence* (Cambridge University Press, Cambridge, UK, 2022).
